# Supplementary material for: Probing few-body nuclear dynamics via 3H and 3He (e,e'p)pn cross-section measurements
Source: arXiv:2001.07230 ancillary file (2020-06-17)
Supplement: Supplementary file 1 [file Supplementary_V6.pdf]

# Supplementary Materials: Probing few-body nuclear dynamics via $^3$H and $^3$He $(e, e'p)$pn cross-section measurements

## 1. CROSS SECTION EXTRACTION

The cross-section was calculated from the $(e, e'p)$ event yield in a given $(p^i_{miss}, E^j_{miss})$ bin as:

$$\sigma(p^i_{miss}, E^j_{miss}) \equiv \frac{d^6\sigma}{dE_e dE_p d\Omega_e d\Omega_p}(p^i_{miss}, E^j_{miss}) = \frac{Yield(p^i_{miss}, E^j_{miss})}{C \cdot t \cdot (\rho/A) \cdot b \cdot V_B \cdot C_{Rad} \cdot C_{BM}}, \quad (1)$$

where all the terms in this equation were defined in the main text. The measured cross sections were corrected for radiative and bin-migration effects, subsequently integrated over $E_{miss}$, and then bin-centered and corrected for tritium decay. The extraction of all correction factors used in Eq. 1 are described and enumerated in the following sections. We then summed over $E_{miss}$ to get the cross section as a a function of $p_{miss}$:

$$\sigma(p^i_{miss}) \equiv \sum_{j=1}^{N} \sigma(p^i_{miss}, E^j_{miss}) \times \Delta E^j_{miss}. \quad (2)$$

The $E_{miss}$ integration limits for each $p_{miss}$ bin are diagrammatically represented in Fig. 1. The exclusion of $E_{miss} > 50$ MeV in the low-$p_{miss}$ kinematical setting comes from the size of radiative corrections (see details in section 1.2). We excluded bins with no measured events and also bins at the edge of our acceptance where the spectrometer modeling is not reliable. Such bins were identified by simulating events with a constant cross section through phase-space and following the same analysis procedure as the data. Bins in which the extracted cross sections (based on the reconstructed simulated events) differed by more than 5% from the input cross-section were excluded.

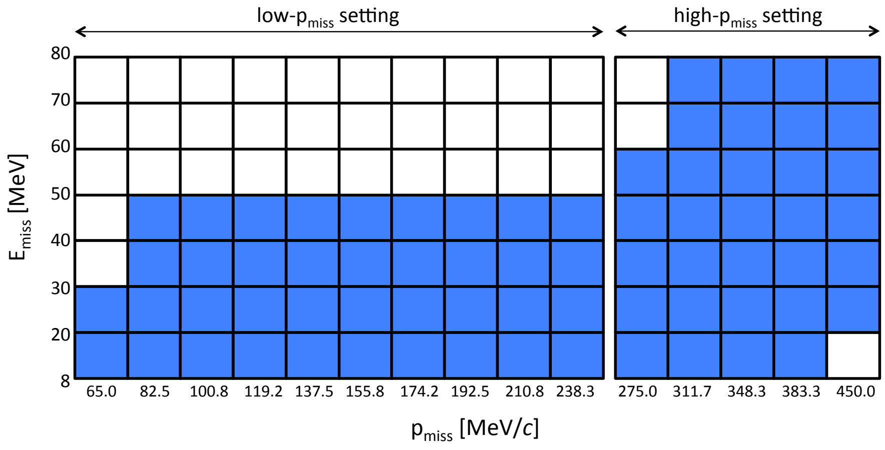


FIG. 1: $E_{miss}$ integration limits for each $p_{miss}$ bin. The blue area indicates the bins that were included in the integration.

### 1.1. Phase-Space and Acceptance Correction Factors

In order to determine the $(e, e'p)$ cross section, the measured normalized yield needs to be corrected for spectrometer acceptance (ACC) and the phase-space volume ($\Phi$) of each $(p_{miss}, E_{miss})$ bin. Both factors are determined from SIMC simulations. ACC is calculated by dividing the total number of events accepted in a given $(p_{miss}, E_{miss})$ bin ($N_{acc}$) by the total number of events generated in that bin ($N$):

$$\text{ACC}(p_{miss}, E_{miss}) = \frac{N_{acc}(p_{miss}, E_{miss})}{N(p_{miss}, E_{miss})} \quad (3)$$

TABLE I: $V_B$ (acceptance-corrected phase-space) correction values in each ($p^i_{miss}, E^j_{miss}$) bin, in unit of MeV$^2$sr$^2$.

| $p_{miss}$ [MeV/$c$] | $E_{miss}$[MeV] 8-20 | 20-30 | 30-40 | 40-50 | 50-60 | 60-70 | 70-80 |
|---|---|---|---|---|---|---|---|
| 36.7 - 73.3 | 1.039e-04 | 4.393e-05 | - | - | - | - | - |
| 73.3 - 91.7 | 2.942e-04 | 1.850e-04 | 1.174e-04 | 6.342e-05 | - | - | - |
| 91.7 - 110.0 | 5.799e-04 | 4.295e-04 | 3.554e-04 | 2.584e-04 | 1.629e-04 | 8.032e-05 | 2.859e-05 |
| 110.0 - 128.3 | 8.562e-04 | 7.015e-04 | 6.665e-04 | 5.735-04 | 4.579e-04 | 3.072e-04 | 1.753e-04 |
| 128.3 - 146.7 | 1.075e-03 | 9.243e-04 | 9.072e-04 | 8.908e-04 | 7.979e-04 | 6.562e-04 | 4.834e-04 |
| 146.7 - 165.0 | 1.262e-03 | 1.075e-03 | 1.086e-03 | 1.092e-03 | 1.043e-03 | 9.231e-04 | 7.830e-04 |
| 165.0 - 183.3 | 1.415e-03 | 1.207e-03 | 1.236e-03 | 1.242e-03 | 1.206e-03 | 1.075e-03 | 9.520e-04 |
| 183.3 - 201.7 | 1.563e-03 | 1.329e-03 | 1.373e-03 | 1.378e-03 | 1.322e-03 | 1.192e-03 | 1.066e-03 |
| 201.7 - 220.0 | 1.636e-03 | 1.420e-03 | 1.465e-03 | 1.497e-03 | 1.439e-03 | 1.287e-03 | 1.151e-03 |
| 220.0 - 256.7 | 2.918e-03 | 2.577e-03 | 2.728e-03 | 2.829e-03 | 2.839e-03 | 2.670e-03 | 2.428e-03 |
| 256.7 - 293.3 | 8.967e-04 | 6.100e-04 | 4.480e-04 | 2.993e-04 | 1.530e-04 | - | - |
| 293.3 - 330.0 | 1.977e-03 | 1.764e-03 | 1.718e-03 | 1.567e-03 | 1.321e-03 | 9.754e-04 | 5.406e-04 |
| 330.0 - 366.7 | 2.635e-03 | 2.481e-03 | 2.525e-03 | 2.516e-03 | 2.453e-03 | 2.355e-03 | 2.111e-03 |
| 366.7 - 400.0 | 2.763e-03 | 2.518e-03 | 2.569e-03 | 2.585e-03 | 2.618e-03 | 2.633e-03 | 2.610e-03 |
| 400.0 - 500.0 | - | 4.878e-03 | 5.302e-03 | 5.734e-03 | 6.135e-03 | 6.568e-03 | 6.982e-03 |

The phase-space volume of a given ($p_{miss}, E_{miss}$) bin, $\Phi$, is calculated by dividing the total number of events generated in that bin by the total number of events generated in the simulation ($N_{tot}$). This is then multiplied by the volume in which the simulated variables were sampled from:

$$\Phi(p_{miss}, E_{miss}) = \frac{N(p_{miss}, E_{miss})}{N_{tot}} \times (\Delta E_e \Delta\Omega_e \Delta E_p \Delta\Omega_p) \tag{4}$$

where the limits on $\Delta E_e$, $\Delta\Omega_e$, $\Delta E_p$, $\Delta\Omega_p$ were larger than the spectrometer acceptance cuts listed in the paper. Since the terms $N(p_{miss}, E_{miss})$ cancel out when multiplying these two corrections, the combined correction factor $V_B$ (see Eq. 1 of main text) was directly determined:

$$V_B(p_{miss}, E_{miss}) \equiv \text{ACC}(p_{miss}, E_{miss}) \cdot \Phi(p_{miss}, E_{miss}) = \frac{N_{acc}(p_{miss}, E_{miss})}{N_{tot}} \times (\Delta E_e \Delta\Omega_e \Delta E_p \Delta\Omega_p) \tag{5}$$

The $V_B$ values used in the cross section extraction are summarized in Table I.

### 1.2. Radiative Corrections

Radiative corrections are determined by running SIMC simulations using the CK+$CC1$ cross section model (see main text for details) with (*Rad*) and without (*Born*) the inclusion of radiative effects. The SIMC radiative-effect model is described in detail in [**?** ]. The radiative correction factor is defined as:

$$C_{Rad}(p_{miss}, E_{miss}) = \frac{Y^{Rad}(p_{miss}, E_{miss})}{Y^{Born}(p_{miss}, E_{miss})} \tag{6}$$

where $Y$ refers to the normalized yield. To determine the relative contributions to the yield from the 2- and 3-body breakup (2bbu and 3bbu respectively) channels in the case of $^3$He, we ran the SIMC simulations for each channel separately (including radiation effects). Subsequently, the simulated data was analyzed using the same event selection cuts as the experimental data. The resulting normalized yield as a function of $E_{miss}$ can be written as:

$$\text{Y}^{Rad}_{^3\text{He}}(E_{miss}) = A\big(\text{Y}^{Rad}_{2bbu}(E_{miss}) + B \cdot \text{Y}^{Rad}_{3bbu}(E_{miss})\big) \tag{7}$$

The two simulated spectra are then simultaneously fitted to the experimental yield, and the coefficients $A$ and $B$ are determined. To avoid the sensitivity coming from the 2bbu channel resolution and position, we binned the 2bbu peak in one bin from $0 - 8$ MeV. The extracted coefficients are summarized in Table II. Fig. 2 shows the resulting $E_{miss}$ distributions for the low- and high-$p_{miss}$ kinematical settings.

TABLE II: Two- and three-body breakup proportionality coefficients for the low- and high-$p_{miss}$ kinematical settings.

| | low-$p_{miss}$ kinematics | high-$p_{miss}$ kinematics |
|---|---|---|
| $A$ | 0.570 ± 0.010 | 0.780 ± 0.095 |
| $B$ | 1.263 ± 0.039 | 1.068 ± 0.147 |

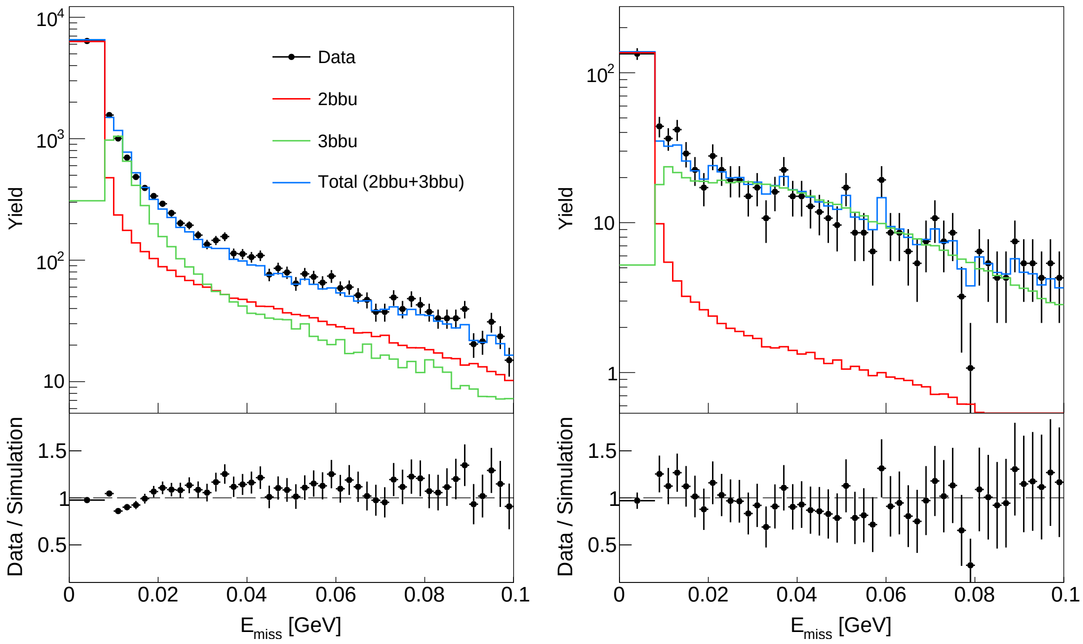


FIG. 2: $^3$He$(e,e'p)$ $E_{miss}$ spectra for the low-$p_{miss}$ (left) and high-$p_{miss}$ (right) kinematical settings. The markers correspond to the measured distribution. The red and green curves correspond to the simulated 2bbu and 3bbu spectra. The blue line corresponds to the total simulated spectrum scaled by $A$ and $B$. The bottom panels show the ratio of the measured to the total simulated spectra.

The radiative correction was applied in 2D $(p_{miss}, E_{miss})$ bin by bin as follows:

$$\sigma^{Born}(p_{miss}, E_{miss}) = \frac{\sigma^{Raw}(p_{miss}, E_{miss})}{C_{Rad}(p_{miss}, E_{miss})} \tag{8}$$

The systematic uncertainty coming from the radiative correction was conservatively assigned to be 10% of the radiative correction size as function of $p_{miss}$ (after integrating over $E_{miss}$) and applied bin by bin.

At large $E_{miss}$, the 3bbu cross section decreased faster than the radiative tail from the 2bbu channel (see Fig. 2). Consequently, the size of the radiative correction depends on the range of $E_{miss}$ integration, as shown in Fig. 3. In the low-$p_{miss}$ kinematical setting, the correction can be very large if we integrate over $E_{miss}$ up to 80 MeV. Hence, in this setting, we integrated up to 50 MeV in order to reduce the radiative correction factor. This effect is smaller for the high-$p_{miss}$ setting, where we integrated up to 80 MeV (see Fig. 1). The size of the correction is shown with other corrections in Fig. 6.

### 1.3. Bin Migration Correction

Bin Migration ($BM$) corrections are determined by running SIMC simulations using the CK+$CC1$ cross section model (see main text for details) with the inclusion of radiative effects. The bin migration correction factor is defined as:

$$C_{BM}(p_{miss}, E_{miss}) = \frac{Y^{Rec.Var}(p_{miss}, E_{miss})}{Y^{Gen.Var}(p_{miss}, E_{miss})}. \tag{9}$$

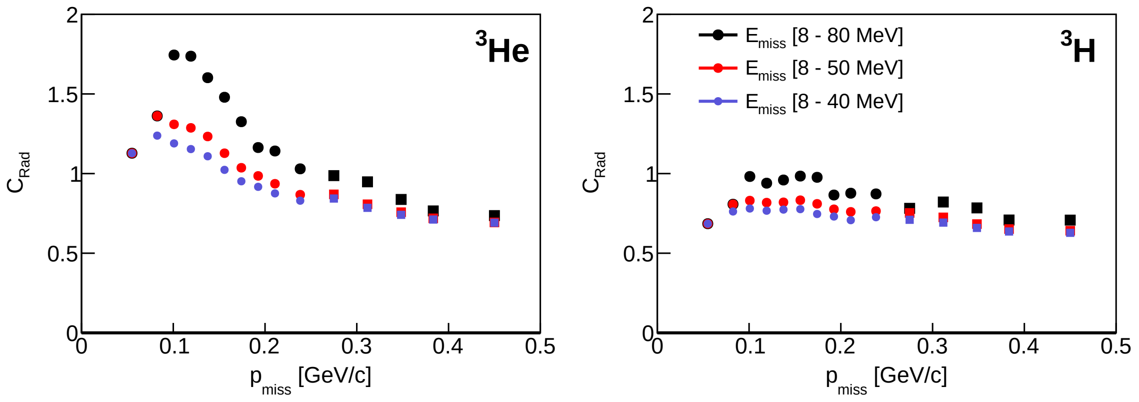


FIG. 3: $C^{Rad}(p_{miss})$ for different ranges of $E_{miss}$ integration for both $^3$He (left) and $^3$H (right). The black, red, and blue distributions correspond to $E_{miss}$ integration in the ranges 8-80, 8-50, and 8-40 MeV respectively.

where $Y^{Rec.Var}$ and $Y^{Gen.Var}$ are the reconstructed normalized yields determined from reconstructed and generated coordinates respectively. For $^3$He, the contribution from the 2bbu and 3bbu is included as described in section 1.2. The bin migration correction was applied in 2D $(p_{miss}, E_{miss})$ bin by bin as follows:

$$\sigma^{Total}(p_{miss}, E_{miss}) = \frac{\sigma^{Born}(p_{miss}, E_{miss})}{C_{BM}(p_{miss}, E_{miss})} \tag{10}$$

The systematic uncertainty coming from bin migration correction was conservatively assigned to be 10% of the correction size as function of $p_{miss}$ (after integrating over $E_{miss}$) and applied bin by bin. The size of the correction is shown with other corrections in Fig. 6.

### 1.4. Bin-Centering Correction

The Bin-Centering ($BC$) correction is defined as ratio of the acceptance-integrated cross section using a given theory model in each $p_{miss}$ bin to the cross section calculated using that same theory model in a single kinematical point within that bin (both integrated over the same range of $E_{miss}$ for a given $p_{miss}$ bin):

$$C_{BC}(p_{miss}) = \frac{\sigma_{integrated}(p_{miss})}{\sigma_{point}(p_{miss})} \tag{11}$$

The point cross section is calculated in a given bin in the kinematical point corresponding to the average values of $Q^2$ and $x_B$ and the central values of $E_{miss}$ and $p_{miss}$ in that bin, and the electron and proton out-of-plane angles $\phi_e = 0°$ and $\phi_p = 180°$. The kinematical points, as well as the point cross sections from different models, are summarized in Tables III and IV for the low- and high-$p_{miss}$ kinematical settings respectively.

The integrated cross section is determined by weighting SIMC events with the same model used to calculate the point cross section, and analyzing these simulated data the same way as the measured data. The integrated cross sections from different models are summarized in Tables V and VI for the low- and high-$p_{miss}$ kinematical settings respectively.

We used both the Cracow and CK+$CC$1 cross-section models for this correction, taking their average as the total correction factor, and their difference as a measure of its uncertainty. Figs. 4 and 5 show the bin centering corrections for the low- and high-$p_{miss}$ kinematical settings respectively. The blue and red curves correspond to the Cracow and CK+$CC$1 corrections respectively. The black markers correspond to the final correction. In the cases in which the fractional error is $< 2\%$, we fixed it at 2%.

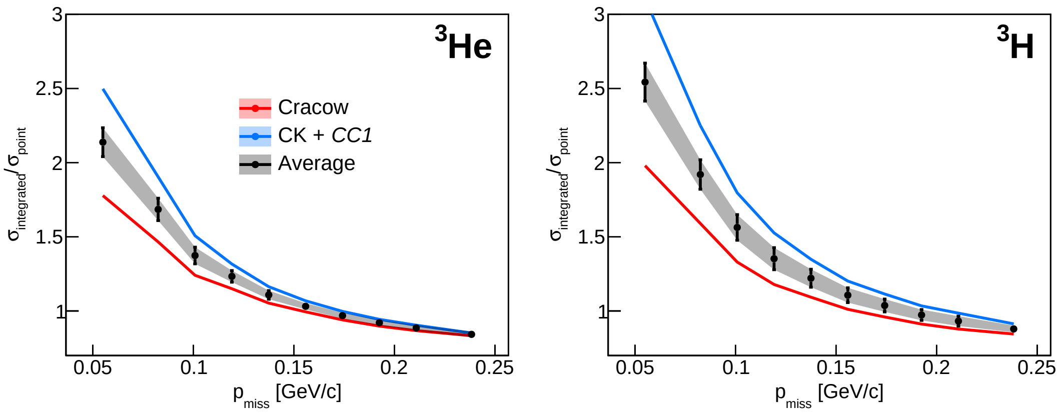


FIG. 4: Bin-centering correction for the low-$p_{miss}$ kinematical setting for $^3$He (left) and $^3$H (right) targets.

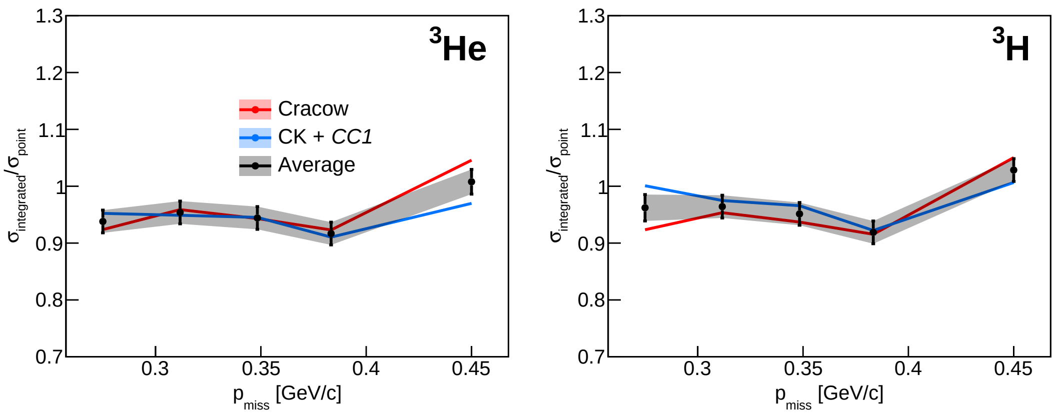


FIG. 5: Same as Fig. 4 in the case of the high-$p_{miss}$ kinematical setting.

### 1.5. Tritium Decay Correction

This experiment was carried out six months after the tritium target cell was filled. Consequently, at that time, a fraction $\epsilon = 2.8\% \pm 0.18\%$ of the total $^3$H nuclei had decayed to $^3$He. Thus, the cross section measured with the $^3$H target ($\sigma^{\mathrm{mixed}}_{^3\mathrm{H}}$) is a mixture of the $^3$H cross section ($\sigma_{^3\mathrm{H}}$) and the $^3$He cross section ($\sigma_{^3\mathrm{He}}$) given by:

$$\sigma^{\mathrm{mixed}}_{^3\mathrm{H}} = (1-\epsilon)\cdot\sigma_{^3\mathrm{H}} + \epsilon\cdot\sigma_{^3\mathrm{He}} \tag{12}$$

Solving for $\sigma_{^3\mathrm{H}}$ we get:

$$\sigma_{^3\mathrm{H}} = \frac{\sigma^{\mathrm{mixed}}_{^3\mathrm{H}} - \epsilon\cdot\sigma_{^3\mathrm{He}}}{1-\epsilon} \tag{13}$$

The decay correction ($DC$) was defined as:

$$C_{DC} \equiv \frac{\sigma^{\mathrm{mixed}}_{^3\mathrm{H}}}{\sigma_{^3\mathrm{H}}} = \frac{1-\epsilon}{1-\epsilon\cdot\frac{\sigma_{^3\mathrm{He}}}{\sigma^{\mathrm{mixed}}_{^3\mathrm{H}}}} \tag{14}$$

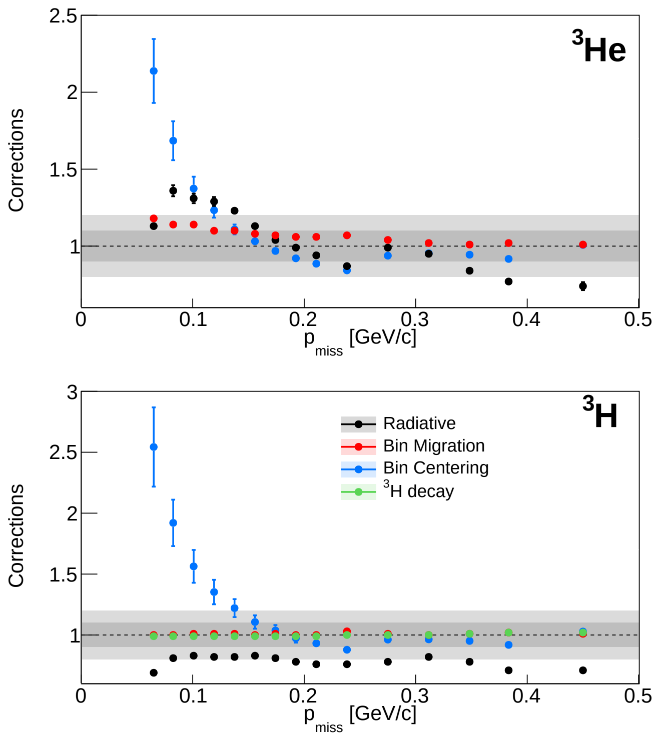


FIG. 6: Corrections applied to the raw cross section to obtain final experimental cross section.

We used the experimental cross section ratio $\sigma_{^3\mathrm{He}}/\sigma^{\mathrm{mixed}}_{^3\mathrm{H}}$ (which includes all the aforementioned corrections) to calculate $C_{DC}$. Error propagation was used to determined the uncertainty of $C_{DC}$ as:

$$\delta C_{DC} = \frac{\epsilon(1-\epsilon)}{(1-\epsilon\cdot\frac{\sigma_{^3\mathrm{He}}}{\sigma^{\mathrm{mixed}}_{^3\mathrm{H}}})^2}\delta\left(\frac{\sigma_{^3\mathrm{He}}}{\sigma^{\mathrm{mixed}}_{^3\mathrm{H}}}\right) \tag{15}$$

Only statistical uncertainties went into the $\delta(\sigma_{^3\mathrm{He}}/\sigma^{\mathrm{mixed}}_{^3\mathrm{H}})$ in the error propagation to avoid double counting the systematic uncertainties. This correction is very small and shown in Fig. 6, with other corrections.

### 1.6. AV18 to CD-Bonn effective conversion

Different cross-section calculations were carried out using different models of the NN interaction. The availability of different models with the CD-Bonn and AV18 NN potentials is summarized in Table VII. However, in order to isolate the differences in the results coming from the details in the different theoretical calculations, we needed to carry out the calculations using the same NN interaction model.

In the absence of two-dimensional cross section calculations of $\sigma(p_{miss}, E_{miss})$ using the same model and both CD-Bonn+TM and AV18+UIX, we used the ratio of one-dimensional momentum distributions $n(p_{miss})$ calculated in [? ] to scale the $E_{miss}$-integrated AV18-based CK+$CC1$ calculation so that we could compare that calculation directly to the Cracow CD-Bonn-based calculation:

$$\sigma^{\mathrm{CD-Bonn}}_{\mathrm{CK}+CC1}(p_{miss}) \equiv \frac{n^{\mathrm{CD-Bonn}}(p_{miss})}{n^{\mathrm{AV18}}(p_{miss})} \times \sigma^{\mathrm{AV18}}_{\mathrm{CK}+CC1}(p_{miss}) \tag{16}$$

Fig. 7 shows the ratio $n^{\mathrm{CD-Bonn}}(k)/n^{\mathrm{AV18}}(k)$ for $^3$He and $^3$H. After this conversion is implemented, all the calculations are based on the CD-Bonn model, and the resulting differences come from the details in the cross-section calculations alone.

TABLE III: Point cross section values and corresponding kinematical points for the low-$p_{miss}$ kinematical setting. The first and second columns correspond to the $p_{miss}$ and $E_{miss}$ values respectively, evaluated at the bin center. The third and fourth columns correspond to weighted-average $x_B$ and $Q^2$ in that $(p^i_{miss}, E^j_{miss})$ bin respectively. The out-of-plane angles for the electron and proton are always fixed at $\phi_e = 0°$ and $\phi_p = 180°$. The remaining columns correspond to the point cross section for $^3$He and $^3$H calculated with the CK+$CC1$ and Cracow models. All the cross sections correspond to $\frac{d^6\sigma}{dE_e d\Omega_e dE_p d\Omega_p}$ and are given in units of $\frac{\text{nb}}{\text{MeV}^2\text{sr}^2}$.

| $p_{miss}$ [MeV/$c$] | $E_{miss}$ [MeV] | $x_B$ | $Q^2$ [(GeV/$c^2$)$^2$] | $^3$He | | $^3$H | |
|---|---|---|---|---|---|---|---|
| | | | | $\sigma_{\text{CK}+CC1}$ | $\sigma_{\text{Cracow}}$ | $\sigma_{\text{CK}+CC1}$ | $\sigma_{\text{Cracow}}$ |
| 65.0 | 14 | 1.08 | 1.74 | 3.277e-02 | 1.797e-02 | 5.270e-02 | 3.547e-02 |
| | 25 | 1.06 | 1.72 | 1.642e-03 | 1.307e-03 | 2.503e-03 | 2.229e-03 |
| 82.5 | 14 | 1.12 | 1.77 | 2.375e-02 | 1.333e-02 | 3.731e-02 | 2.539e-02 |
| | 25 | 1.09 | 1.75 | 1.439e-03 | 1.116e-03 | 2.128e-03 | 1.863e-03 |
| | 35 | 1.07 | 1.74 | 2.695e-04 | 2.350e-04 | 3.714e-04 | 3.475e-04 |
| | 45 | 1.04 | 1.72 | 7.805e-05 | 7.643e-05 | 8.745e-05 | 9.245e-05 |
| 100.8 | 14 | 1.15 | 1.80 | 1.672e-02 | 9.678e-03 | 2.560e-02 | 1.768e-02 |
| | 25 | 1.12 | 1.79 | 1.216e-03 | 9.191e-04 | 1.734e-03 | 1.481e-03 |
| | 35 | 1.10 | 1.77 | 2.520e-04 | 2.091e-04 | 3.385e-04 | 3.061e-04 |
| | 45 | 1.07 | 1.75 | 7.584e-05 | 7.007e-05 | 8.649e-05 | 8.575e-05 |
| 119.2 | 14 | 1.18 | 1.84 | 1.100e-02 | 6.616e-03 | 1.637e-02 | 1.156e-02 |
| | 25 | 1.15 | 1.82 | 1.027e-03 | 7.620e-04 | 1.409e-03 | 1.174e-03 |
| | 35 | 1.13 | 1.80 | 2.321e-04 | 1.855e-04 | 3.029e-04 | 2.637e-04 |
| | 45 | 1.10 | 1.79 | 7.120e-05 | 6.214e-05 | 8.191e-05 | 7.691e-05 |
| 137.5 | 14 | 1.21 | 1.88 | 7.074e-03 | 4.416e-03 | 1.026e-02 | 7.373e-03 |
| | 25 | 1.18 | 1.86 | 8.358e-04 | 6.117e-04 | 1.107e-03 | 9.011e-04 |
| | 35 | 1.16 | 1.85 | 2.015e-04 | 1.562e-04 | 2.559e-04 | 2.143e-04 |
| | 45 | 1.13 | 1.83 | 6.611e-05 | 5.513e-05 | 7.637e-05 | 6.799e-05 |
| 155.8 | 14 | 1.24 | 1.93 | 4.301e-03 | 2.805e-03 | 6.075e-03 | 4.475e-03 |
| | 25 | 1.21 | 1.91 | 6.519e-04 | 4.738e-04 | 8.362e-04 | 6.702e-04 |
| | 35 | 1.19 | 1.90 | 1.729e-04 | 1.308e-04 | 2.140e-04 | 1.735e-04 |
| | 45 | 1.16 | 1.88 | 5.936e-05 | 4.761e-05 | 6.860e-05 | 5.774e-05 |
| 174.2 | 14 | 1.27 | 1.98 | 2.542e-03 | 1.742e-03 | 3.498e-03 | 2.657e-03 |
| | 25 | 1.24 | 1.96 | 4.965e-04 | 3.615e-04 | 6.198e-04 | 4.932e-04 |
| | 35 | 1.22 | 1.95 | 1.459e-04 | 1.086e-04 | 1.770e-04 | 1.400e-04 |
| | 45 | 1.19 | 1.93 | 5.274e-05 | 4.095e-05 | 6.099e-05 | 4.885e-05 |
| 192.5 | 14 | 1.30 | 2.03 | 1.461e-03 | 1.058e-03 | 1.958e-03 | 1.548e-03 |
| | 25 | 1.27 | 2.01 | 3.687e-04 | 2.712e-04 | 4.505e-04 | 3.580e-04 |
| | 35 | 1.24 | 2.00 | 1.230e-04 | 9.065e-05 | 1.470e-04 | 1.144e-04 |
| | 45 | 1.22 | 1.98 | 4.632e-05 | 3.504e-05 | 5.369e-05 | 4.150e-05 |
| 210.8 | 14 | 1.33 | 2.08 | 8.181e-04 | 6.305e-04 | 1.067e-03 | 8.853e-04 |
| | 25 | 1.30 | 2.06 | 2.658e-04 | 1.994e-04 | 3.195e-04 | 2.555e-04 |
| | 35 | 1.27 | 2.05 | 1.004e-04 | 7.377e-05 | 1.188e-04 | 9.164e-05 |
| | 45 | 1.25 | 2.03 | 4.019e-05 | 2.983e-05 | 4.677e-05 | 3.533e-05 |
| 238.3 | 14 | 1.36 | 2.13 | 3.686e-04 | 2.999e-04 | 4.630e-04 | 3.965e-04 |
| | 25 | 1.34 | 2.12 | 1.604e-04 | 1.240e-04 | 1.900e-04 | 1.529e-04 |
| | 35 | 1.31 | 2.11 | 7.422e-05 | 5.450e-05 | 8.740e-05 | 6.652e-05 |
| | 45 | 1.29 | 2.10 | 3.236e-05 | 2.362e-05 | 3.806e-05 | 2.812e-05 |

## 2. FINAL RESULTS

The resulting cross sections as a function of $p_{miss}$ are summarized in Tables VIII and IX for $^3$He and $^3$H respectively. We also include Figs. 8 and 9 which are equivalent to Figs. 2 and 3 from the main text respectively, with the distinction that, in the plots presented here, the theoretical cross sections from the denominators are the acceptance-integrated cross sections determined by propagating these calculations through a SIMC simulation, and subsequently following the analysis used in data. In this case, bin-centering corrections cancel. Only statistical uncertainties are shown. In the case of tritium, the decay correction is not included.

TABLE IV: Same as Table III for the high-$p_{miss}$ kinematical setting. The point cross section using the Sargsian-FSI model is also included.

| $p_{miss}$ [MeV/$c$] | $E_{miss}$ [MeV] | $x_B$ | $Q^2$ [(GeV/$c^2$)$^2$] | $^3$He $\sigma_{\mathrm{CK}+CC1}$ | $^3$He $\sigma_{\mathrm{Cracow}}$ | $^3$He $\sigma_{\mathrm{Sargsian-FSI}}$ | $^3$H $\sigma_{\mathrm{CK}+CC1}$ | $^3$H $\sigma_{\mathrm{Cracow}}$ | $^3$H $\sigma_{\mathrm{Sargsian-FSI}}$ |
|---|---|---|---|---|---|---|---|---|---|
| 275.0 | 14 | 1.46 | 1.85 | 2.192e-04 | 2.071e-04 | 2.171e-04 | 2.575e-04 | 2.528e-04 | 1.362e-04 |
| | 25 | 1.43 | 1.84 | 1.476e-04 | 1.232e-04 | 2.068e-04 | 1.731e-04 | 1.456e-04 | 1.569e-04 |
| | 35 | 1.40 | 1.82 | 9.611e-05 | 7.180e-05 | 1.314e-04 | 1.139e-04 | 8.603e-05 | 9.966e-05 |
| | 45 | 1.36 | 1.81 | 5.081e-05 | 3.693e-05 | 6.730e-05 | 6.097e-05 | 4.421e-05 | 5.117e-05 |
| | 55 | 1.34 | 1.80 | 2.606e-05 | 1.868e-05 | 3.360e-05 | 3.130e-05 | 2.200e-05 | 2.545e-05 |
| 311.7 | 14 | 1.52 | 1.92 | 6.947e-05 | 6.653e-05 | 5.879e-05 | 7.472e-05 | 7.416e-05 | 4.102e-05 |
| | 25 | 1.49 | 1.90 | 6.510e-05 | 5.490e-05 | 7.181e-05 | 7.553e-05 | 6.249e-05 | 5.702e-05 |
| | 35 | 1.45 | 1.88 | 5.764e-05 | 4.183e-05 | 6.227e-05 | 6.887e-05 | 4.933e-05 | 5.198e-05 |
| | 45 | 1.42 | 1.86 | 3.887e-05 | 2.634e-05 | 3.929e-05 | 4.728e-05 | 3.162e-05 | 3.314e-05 |
| | 55 | 1.39 | 1.85 | 2.255e-05 | 1.456e-05 | 2.206e-05 | 2.770e-05 | 1.758e-05 | 1.859e-05 |
| | 65 | 1.36 | 1.84 | 1.383e-05 | 8.127e-06 | 1.283e-05 | 1.688e-05 | 9.612e-06 | 1.063e-05 |
| | 75 | 1.34 | 1.82 | 8.528e-06 | 4.702e-06 | 7.604e-06 | 1.022e-05 | 5.321e-06 | 6.084e-06 |
| 348.3 | 14 | 1.58 | 2.00 | 2.107e-05 | 2.060e-05 | 1.385e-05 | 1.834e-05 | 2.041e-05 | 9.079e-06 |
| | 25 | 1.55 | 1.98 | 2.679e-05 | 2.170e-05 | 2.374e-05 | 2.972e-05 | 2.374e-05 | 2.058e-05 |
| | 35 | 1.51 | 1.96 | 3.107e-05 | 2.087e-05 | 2.647e-05 | 3.672e-05 | 2.420e-05 | 2.419e-05 |
| | 45 | 1.48 | 1.94 | 2.722e-05 | 1.602e-05 | 2.286e-05 | 3.286e-05 | 1.920e-05 | 2.049e-05 |
| | 55 | 1.44 | 1.92 | 1.925e-05 | 1.036e-05 | 1.561e-05 | 2.349e-05 | 1.263e-05 | 1.382e-05 |
| | 65 | 1.41 | 1.90 | 1.269e-05 | 6.283e-06 | 1.011e-05 | 1.548e-05 | 7.613e-06 | 8.709e-06 |
| | 75 | 1.38 | 1.88 | 8.413e-06 | 3.908e-06 | 6.760e-06 | 1.017e-05 | 4.626e-06 | 5.552e-06 |
| 383.3 | 14 | 1.65 | 2.10 | 8.128e-06 | 6.359e-06 | 3.431e-06 | 4.939e-06 | 5.317e-06 | 2.500e-06 |
| | 25 | 1.61 | 2.07 | 1.263e-05 | 8.332e-06 | 8.336e-06 | 1.277e-05 | 8.663e-06 | 7.540e-06 |
| | 35 | 1.57 | 2.05 | 1.719e-05 | 9.872e-06 | 1.198e-05 | 1.941e-05 | 1.120e-05 | 1.084e-05 |
| | 45 | 1.54 | 2.03 | 1.845e-05 | 9.038e-06 | 1.296e-05 | 2.141e-05 | 1.073e-05 | 1.204e-05 |
| | 55 | 1.50 | 2.01 | 1.565e-05 | 6.707e-06 | 1.057e-05 | 1.832e-05 | 8.137e-06 | 9.594e-06 |
| | 65 | 1.47 | 1.99 | 1.143e-05 | 4.517e-06 | 7.580e-06 | 1.338e-05 | 5.490e-06 | 6.672e-06 |
| | 75 | 1.43 | 1.97 | 8.141e-06 | 2.996e-06 | 5.503e-06 | 9.466e-06 | 3.603e-06 | 4.603e-06 |
| 450.0 | 25 | 1.70 | 2.20 | 4.287e-06 | 1.672e-06 | 1.536e-06 | 3.142e-06 | 1.490e-06 | 1.618e-06 |
| | 35 | 1.66 | 2.18 | 6.255e-06 | 2.392e-06 | 2.725e-06 | 5.916e-06 | 2.543e-06 | 2.860e-06 |
| | 45 | 1.62 | 2.17 | 8.534e-06 | 2.841e-06 | 3.840e-06 | 8.696e-06 | 3.226e-06 | 3.923e-06 |
| | 55 | 1.59 | 2.15 | 9.692e-06 | 2.727e-06 | 4.409e-06 | 1.005e-05 | 3.176e-06 | 4.135e-06 |
| | 65 | 1.56 | 2.14 | 9.057e-06 | 2.280e-06 | 4.262e-06 | 9.375e-06 | 2.684e-06 | 3.780e-06 |
| | 75 | 1.53 | 2.13 | 7.733e-06 | 1.752e-06 | 3.598e-06 | 7.957e-06 | 2.067e-06 | 3.055e-06 |

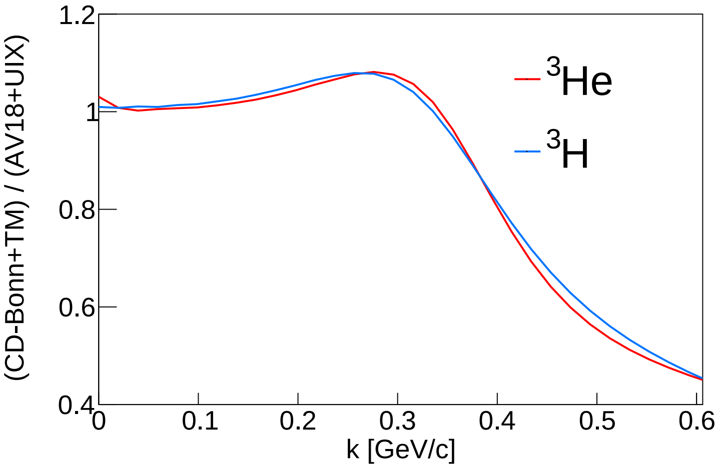


FIG. 7: Ratio of the $^3$He and $^3$H proton momentum distributions obtained using the CD-Bonn+TM potential relative to that obtained using AV18+UIX potential using the calculations of Ref. [**?** ].

TABLE V: Acceptance-integrated cross section values and corresponding kinematical points for the low-$p_{miss}$ kinematical setting. The first and second columns correspond to the $p_{miss}$ and $E_{miss}$ bin ranges respectively. The third and fourth columns correspond to weighted-average $x_B$ and $Q^2$ in that $(p^i_{miss}, E^j_{miss})$ bin respectively. The remaining columns correspond to the integrated cross section for $^3$He and $^3$H calculated with the CK+$CC1$ and Cracow models. All the cross sections correspond to $\frac{d^6\sigma}{dE_e d\Omega_e dE_p d\Omega_p}$ and are given in units of $\frac{\text{nb}}{\text{MeV}^2\text{sr}^2}$.

| $p_{miss}$ [MeV/$c$] | $E_{miss}$ [MeV] | $x_B$ | $Q^2$ [(GeV/$c^2$)$^2$] | $^3$He | | $^3$H | |
|---|---|---|---|---|---|---|---|
| | | | | $\sigma_{\text{CK}+CC1}$ | $\sigma_{\text{Cracow}}$ | $\sigma_{\text{CK}+CC1}$ | $\sigma_{\text{Cracow}}$ |
| 36.7 - 73.3 | 8 - 20 | 1.08 | 1.74 | 8.329e-02 | 3.224e-02 | 1.674e-01 | 7.167e-02 |
| | 20 - 30 | 1.06 | 1.72 | 2.370e-03 | 1.976e-03 | 3.302e-03 | 2.673e-03 |
| 73.3 - 91.7 | 8 - 20 | 1.12 | 1.77 | 4.632e-02 | 1.981e-02 | 8.612e-02 | 4.119e-02 |
| | 20 - 30 | 1.09 | 1.75 | 1.665e-03 | 1.375e-03 | 2.587e-03 | 2.100e-03 |
| | 30 - 40 | 1.07 | 1.74 | 3.253e-04 | 3.035e-04 | 4.962e-04 | 4.529e-04 |
| | 40 - 50 | 1.04 | 1.72 | 8.014e-05 | 8.280e-05 | 1.318e-04 | 1.357e-04 |
| 91.7 - 110.0 | 8 - 20 | 1.15 | 1.80 | 2.572e-02 | 1.206e-02 | 4.711e-02 | 2.386e-02 |
| | 20 -30 | 1.12 | 1.79 | 1.360e-03 | 1.099e-03 | 2.084e-03 | 1.662e-03 |
| | 30 -40 | 1.10 | 1.77 | 2.751e-04 | 2.462e-04 | 3.650e-04 | 3.236e-04 |
| | 40 - 50 | 1.07 | 1.75 | 8.430e-05 | 8.259e-05 | 8.832e-05 | 8.644e-05 |
| 110.0 - 128.3 | 8 - 20 | 1.18 | 1.84 | 1.482e-02 | 7.661e-03 | 2.560e-02 | 1.377e-02 |
| | 20 - 30 | 1.15 | 1.82 | 1.061e-03 | 8.468e-04 | 1.617e-03 | 1.274e-03 |
| | 30 - 40 | 1.13 | 1.80 | 2.130e-04 | 1.842e-04 | 3.031e-04 | 2.605e-04 |
| | 40 - 50 | 1.10 | 1.79 | 7.212e-05 | 6.699e-05 | 8.331e-05 | 7.751e-05 |
| 128.3 - 146.7 | 8 - 20 | 1.21 | 1.88 | 8.438e-03 | 4.678e-03 | 1.423e-02 | 8.167e-03 |
| | 20 - 30 | 1.18 | 1.86 | 7.810e-04 | 6.154e-04 | 1.136e-03 | 8.837e-04 |
| | 30 - 40 | 1.16 | 1.85 | 1.919e-04 | 1.612e-04 | 2.608e-04 | 2.166e-04 |
| | 40 - 50 | 1.13 | 1.83 | 6.414e-05 | 5.692e-05 | 7.241e-05 | 6.395e-05 |
| 146.7 - 165.0 | 8 - 20 | 1.24 | 1.93 | 4.704e-03 | 2.781e-03 | 7.489e-03 | 4.556e-03 |
| | 20 - 30 | 1.21 | 1.91 | 6.010e-04 | 4.794e-04 | 8.393e-04 | 6.485e-04 |
| | 30 - 40 | 1.19 | 1.90 | 1.602e-04 | 1.310e-04 | 2.095e-04 | 1.687e-04 |
| | 40 - 50 | 1.16 | 1.88 | 5.500e-05 | 4.694e-05 | 6.931e-05 | 5.804e-05 |
| 165.0 - 183.3 | 8 - 20 | 1.27 | 1.98 | 2.589e-03 | 1.622e-03 | 4.012e-03 | 2.564e-03 |
| | 20 - 30 | 1.24 | 1.96 | 4.471e-04 | 3.502e-04 | 5.961e-04 | 4.615e-04 |
| | 30 - 40 | 1.22 | 1.95 | 1.336e-04 | 1.074e-04 | 1.674e-04 | 1.320e-04 |
| | 40 - 50 | 1.19 | 1.93 | 4.845e-05 | 3.998e-05 | 5.581e-05 | 4.455e-05 |
| 183.3 - 201.7 | 8 - 20 | 1.30 | 2.03 | 1.418e-03 | 9.436e-04 | 2.088e-03 | 1.414e-03 |
| | 20 - 30 | 1.27 | 2.01 | 3.126e-04 | 2.466e-04 | 4.167e-04 | 3.243e-04 |
| | 30 - 40 | 1.24 | 2.00 | 1.072e-04 | 8.507e-05 | 1.311e-04 | 1.018e-04 |
| | 40 - 50 | 1.22 | 1.98 | 4.074e-05 | 3.272e-05 | 5.046e-05 | 3.893e-05 |
| 201.7 - 220.0 | 8 - 20 | 1.33 | 2.08 | 7.642e-04 | 5.418e-04 | 1.095e-03 | 7.808e-04 |
| | 20 - 30 | 1.30 | 2.06 | 2.209e-04 | 1.765e-04 | 2.811e-04 | 2.212e-04 |
| | 30 - 40 | 1.27 | 2.05 | 8.217e-05 | 6.484e-05 | 1.021e-04 | 7.861e-05 |
| | 40 - 50 | 1.25 | 2.03 | 3.505e-05 | 2.759e-05 | 4.258e-05 | 3.211e-05 |
| 220.0 - 256.7 | 8 - 20 | 1.36 | 2.13 | 3.271e-04 | 2.489e-04 | 4.442e-04 | 3.379e-04 |
| | 20 - 30 | 1.34 | 2.12 | 1.268e-04 | 1.039e-04 | 1.582e-04 | 1.269e-04 |
| | 30 -40 | 1.31 | 2.11 | 5.801e-05 | 4.548e-05 | 7.159e-05 | 5.456e-05 |
| | 40 -50 | 1.29 | 2.10 | 2.640e-05 | 2.037e-05 | 3.248e-05 | 2.397e-05 |

TABLE VI: Same as Table V for the high-$p_{miss}$ kinematical setting. The acceptance-integrated cross section using the Sargsian-FSI model is also included.

| $p_{miss}$ [MeV/$c$] | $E_{miss}$ [MeV] | $x_B$ | $Q^2$ [(GeV/$c^2$)$^2$] | $^3$He | | | $^3$H | | |
|---|---|---|---|---|---|---|---|---|---|
| | | | | $\sigma_{\mathrm{CK}+CC1}$ | $\sigma_{\mathrm{Cracow}}$ | $\sigma_{\mathrm{Sargsian-FSI}}$ | $\sigma_{\mathrm{CK}+CC1}$ | $\sigma_{\mathrm{Cracow}}$ | $\sigma_{\mathrm{Sargsian-FSI}}$ |
| 256.7 - 293.3 | 8 - 20 | 1.46 | 1.85 | 2.205e-04 | 1.884e-04 | 1.845e-04 | 2.763e-04 | 2.319e-04 | 1.2307e-04 |
| | 20 - 30 | 1.43 | 1.84 | 1.274e-04 | 1.100e-04 | 1.892e-04 | 1.545e-04 | 1.289e-04 | 1.3005e-04 |
| | 30 - 40 | 1.40 | 1.82 | 8.984e-05 | 7.018e-05 | 1.379e-04 | 1.115e-04 | 8.376e-05 | 8.879e-05 |
| | 40 - 50 | 1.36 | 1.81 | 4.837e-05 | 3.628e-05 | 5.939e-05 | 5.916e-05 | 4.225e-05 | 4.859e-05 |
| | 50 - 60 | 1.34 | 1.80 | 2.549e-05 | 1.861e-05 | 3.446e-05 | 3.207e-05 | 2.200e-05 | 2.643e-05 |
| 293.3 - 330.0 | 8 - 20 | 1.52 | 1.92 | 6.810e-05 | 6.309e-05 | 4.735e-05 | 7.761e-05 | 7.158e-05 | 3.512e-05 |
| | 20 - 30 | 1.49 | 1.90 | 6.038e-05 | 5.230e-05 | 6.815e-05 | 7.019e-05 | 5.832e-05 | 5.313e-05 |
| | 30 - 40 | 1.45 | 1.88 | 5.339e-05 | 4.018e-05 | 5.762e-05 | 6.468e-05 | 4.637e-05 | 5.052e-05 |
| | 40 - 50 | 1.42 | 1.86 | 3.609e-05 | 2.525e-05 | 3.859e-05 | 4.475e-05 | 2.967e-05 | 2.915e-05 |
| | 50 - 60 | 1.39 | 1.85 | 2.188e-05 | 1.454e-05 | 2.075e-05 | 2.790e-05 | 1.746e-05 | 2.020e-05 |
| | 60 - 70 | 1.36 | 1.84 | 1.391e-05 | 8.480e-06 | 1.460e-05 | 1.671e-05 | 9.520e-06 | 9.560e-06 |
| | 70 - 80 | 1.34 | 1.82 | 7.693e-06 | 4.360e-06 | 6.180e-06 | 1.032e-05 | 5.380e-06 | 6.330e-06 |
| 330.0 - 366.7 | 8 - 20 | 1.58 | 2.00 | 2.090e-05 | 1.895e-05 | 1.241e-05 | 1.990e-05 | 1.907e-05 | 8.760e-06 |
| | 20 - 30 | 1.55 | 1.98 | 2.591e-05 | 2.058e-05 | 2.393e-05 | 2.835e-05 | 2.196e-05 | 1.993e-05 |
| | 30 - 40 | 1.51 | 1.96 | 2.942e-05 | 1.995e-05 | 2.511e-05 | 3.517e-05 | 2.291e-05 | 2.454e-05 |
| | 40 - 50 | 1.48 | 1.94 | 2.488e-05 | 1.507e-05 | 2.162e-05 | 3.048e-05 | 1.775e-05 | 1.931e-05 |
| | 50 - 60 | 1.44 | 1.92 | 1.785e-05 | 9.940e-06 | 1.613e-05 | 2.243e-05 | 1.202e-05 | 1.342e-05 |
| | 60 - 70 | 1.41 | 1.90 | 1.196e-05 | 6.160e-06 | 8.840e-06 | 1.490e-05 | 7.350e-06 | 8.210e-06 |
| | 70 - 80 | 1.38 | 1.88 | 7.350e-06 | 3.520e-06 | 6.240e-06 | 9.404e-06 | 4.280e-06 | 5.680e-06 |
| 366.7 - 400.0 | 8 - 20 | 1.65 | 2.10 | 7.467e-06 | 5.780e-06 | 3.300e-06 | 4.991e-06 | 4.930e-06 | 2.460e-06 |
| | 20 - 30 | 1.61 | 2.07 | 1.167e-05 | 7.720e-06 | 7.010e-06 | 1.144e-05 | 7.810e-06 | 6.250e-06 |
| | 30 - 40 | 1.57 | 2.05 | 1.578e-05 | 9.090e-06 | 9.840e-06 | 1.786e-05 | 1.027e-05 | 8.670e-06 |
| | 40 - 50 | 1.54 | 2.03 | 1.686e-05 | 8.410e-06 | 1.294e-05 | 1.967e-05 | 9.810e-06 | 1.082e-05 |
| | 50 - 60 | 1.50 | 2.01 | 1.422e-05 | 6.270e-06 | 9.010e-06 | 1.689e-05 | 7.480e-06 | 9.220e-06 |
| | 60 - 70 | 1.47 | 1.99 | 1.047e-05 | 4.260e-06 | 7.810e-06 | 1.244e-05 | 5.090e-06 | 6.320e-06 |
| | 70 - 80 | 1.43 | 1.97 | 6.935e-06 | 2.630e-06 | 5.160e-06 | 8.549e-06 | 3.250e-06 | 4.300e-06 |
| 400.0 - 500.0 | 20 - 30 | 1.70 | 2.20 | 5.097e-06 | 2.160e-06 | 1.750e-06 | 4.104e-06 | 2.020e-06 | 1.900e-06 |
| | 30 - 40 | 1.66 | 2.18 | 7.108e-06 | 2.820e-06 | 3.830e-06 | 7.091e-06 | 3.060e-06 | 3.320e-06 |
| | 40 - 50 | 1.62 | 2.17 | 8.889e-06 | 3.050e-06 | 4.450e-06 | 9.327e-06 | 3.470e-06 | 3.580e-06 |
| | 50 - 60 | 1.59 | 2.15 | 9.166e-06 | 2.700e-06 | 4.130e-06 | 9.812e-06 | 3.150e-06 | 4.090e-06 |
| | 60 - 70 | 1.56 | 2.14 | 8.014e-06 | 2.130e-06 | 3.720e-06 | 8.547e-06 | 2.500e-06 | 3.600e-06 |
| | 70 - 80 | 1.53 | 2.13 | 5.911e-06 | 1.430e-06 | 3.050e-06 | 6.547e-06 | 1.750e-06 | 2.440e-06 |

TABLE VII: NN potentials used in the different calculations.

| | Cracow | CK+$CC1$ | Sargsian-FSI |
|---|---|---|---|
| CD-Bonn | ✓ | | ✓ |
| AV18 | | ✓ | ✓ |

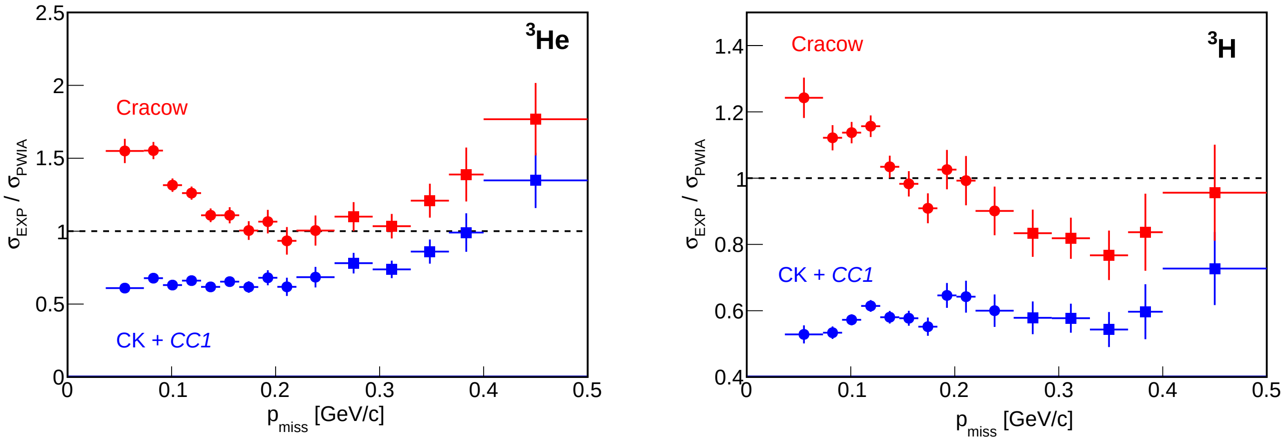


FIG. 8: Plots equivalent to Fig. 2 in the main text, but in this case the theoretical cross section from the denominator is extracted following the acceptance-integrated cross section method used in data.

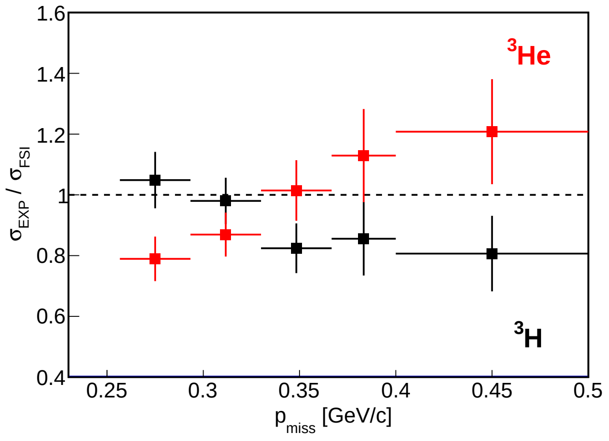


FIG. 9: Plots equivalent to Fig. 3 in the main text, but in this case the theoretical cross section from the denominator is extracted following the acceptance-integrated cross section method used in data.

## 3. EFFECT OF INTERACTION BETWEEN THE TWO SPECTATOR NUCLEONS ($FSI_{23}$)

Fig. 10 shows the $^3$He missing energy distribution for both kinematical settings calculated with and without the inclusion of the continuum interaction between the two spectator nucleons ($FSI_{23}$). This effect is larger in the low-$p_{miss}$ kinematical setting.

TABLE VIII: Values of the $E_{miss}$-integrated $^3$He experimental cross section and the corrections from Figure 2 in the main text. The first column corresponds to the $p_{miss}$value at the bin center. The second column corresponds to measured cross section after all corrections with corresponding statistical uncertainty. The third, fourth, and fifth columns correspond to bin-centering, radiative and bin-migration corrections with their corresponding point-to-point uncertainty, respectively. The sixth column corresponds to cut sensitivity point-to-point uncertainty in %. The seventh column corresponds to the total point-to-point uncertainty.

| $p_{miss}$ [MeV/$c$] | $\sigma$ ± Stat. Unc. [$\frac{\text{nb}}{\text{sr}^2\text{MeV}}$] | Bin Centering | Radiative Correction | Bin Migration | Cut Sens. [%] | Total Uncertainty |
|---|---|---|---|---|---|---|
| 65.0 | (2.948 ± 0.135)e-01 | 2.14 ± 0.208 | 1.13 ± 0.013 | 1.18 ± 0.018 | 3.47 | 3.376e-02 |
| 82.5 | (2.353 ± 0.080)e-01 | 1.68 ± 0.127 | 1.36 ± 0.036 | 1.14 ± 0.014 | 1.54 | 2.091e-02 |
| 100.8 | (1.522 ± 0.050)e-01 | 1.37 ± 0.070 | 1.31 ± 0.031 | 1.14 ± 0.014 | 1.39 | 1.090e-02 |
| 119.2 | (1.052 ± 0.036)e-01 | 1.23 ± 0.048 | 1.29 ± 0.029 | 1.10 ± 0.011 | 1.58 | 6.281e-03 |
| 137.5 | (6.450 ± 0.268)e-02 | 1.11 ± 0.032 | 1.23 ± 0.023 | 1.10 ± 0.011 | 1.11 | 3.608e-03 |
| 155.8 | (4.295 ± 0.212)e-02 | 1.03 ± 0.021 | 1.13 ± 0.013 | 1.08 ± 0.011 | 1.27 | 2.455e-03 |
| 174.2 | (2.535 ± 0.161)e-02 | 0.97 ± 0.017 | 1.04 ± 0.004 | 1.07 ± 0.011 | 2.30 | 1.790e-03 |
| 192.5 | (1.732 ± 0.131)e-02 | 0.92 ± 0.013 | 0.99 ± 0.001 | 1.06 ± 0.011 | 3.00 | 1.441e-03 |
| 210.8 | (9.688 ± 0.980)e-03 | 0.89 ± 0.011 | 0.94 ± 0.006 | 1.06 ± 0.011 | 5.13 | 1.110e-03 |
| 238.3 | (5.584 ± 0.574)e-03 | 0.84 ± 0.010 | 0.87 ± 0.013 | 1.07 ± 0.011 | 5.85 | 6.708e-04 |
| 275.0 | (5.405 ± 0.488)e-03 | 0.94 ± 0.019 | 0.93 ± 0.007 | 1.04 ± 0.010 | 8.28 | 6.732e-04 |
| 311.7 | (2.394 ± 0.195)e-03 | 0.95 ± 0.019 | 0.95 ± 0.005 | 1.02 ± 0.010 | 3.73 | 2.211e-04 |
| 348.3 | (1.255 ± 0.121)e-03 | 0.94 ± 0.019 | 0.84 ± 0.016 | 1.01 ± 0.010 | 3.42 | 1.334e-04 |
| 383.3 | (6.865 ± 0.914)e-04 | 0.92 ± 0.018 | 0.77 ± 0.023 | 1.02 ± 0.010 | 5.27 | 1.016e-04 |
| 450.0 | (2.508 ± 0.353)e-04 | 1.01 ± 0.022 | 0.74 ± 0.026 | 1.01 ± 0.010 | 4.68 | 3.867e-05 |

TABLE IX: Same as Table VIII for $^3$H. The $^3$H decay correction and corresponding point-to-point uncertainty are also included.

| $p_{miss}$ [MeV/$c$] | $\sigma$ ± Stat. Unc. [$\frac{\text{nb}}{\text{sr}^2\text{MeV}}$] | Bin Centering | Radiative Correction | Bin Migration | Cut Sens. [%] | $^3$H decay | Total Uncertainty |
|---|---|---|---|---|---|---|---|
| 65.0 | (4.376 ± 0.170)e-01 | 2.54 ± 0.325 | 0.69 ± 0.031 | 1.00 ± 0.01 | 2.79 | 0.99 ± 0.001 | 6.306e-02 |
| 82.5 | (3.075 ± 0.089)e-01 | 1.92 ± 0.190 | 0.81 ± 0.019 | 1.00 ± 0.01 | 2.02 | 0.99 ± 0.001 | 3.332e-02 |
| 100.8 | (2.256 ± 0.057)e-01 | 1.56 ± 0.135 | 0.83 ± 0.017 | 1.01 ± 0.01 | 1.39 | 0.99 ± 0.001 | 2.115e-02 |
| 119.2 | (1.566 ± 0.041)e-01 | 1.35 ± 0.100 | 0.82 ± 0.018 | 1.01 ± 0.01 | 2.07 | 0.99 ± 0.001 | 1.330e-02 |
| 137.5 | (9.383 ± 0.294)e-02 | 1.22 ± 0.074 | 0.82 ± 0.018 | 1.01 ± 0.01 | 1.84 | 0.99 ± 0.001 | 6.992e-03 |
| 155.8 | (5.690 ± 0.217)e-02 | 1.11 ± 0.054 | 0.83 ± 0.017 | 1.00 ± 0.01 | 2.48 | 0.99 ± 0.001 | 4.049e-03 |
| 174.2 | (3.289 ± 0.162)e-02 | 1.04 ± 0.045 | 0.81 ± 0.019 | 1.01 ± 0.01 | 2.46 | 0.99 ± 0.002 | 2.447e-03 |
| 192.5 | (2.302 ± 0.133)e-02 | 0.97 ± 0.035 | 0.78 ± 0.022 | 1.00 ± 0.01 | 2.82 | 0.99 ± 0.002 | 1.833e-03 |
| 210.8 | (1.365 ± 0.102)e-02 | 0.93 ± 0.031 | 0.76 ± 0.024 | 1.00 ± 0.01 | 3.07 | 0.99 ± 0.002 | 1.276e-03 |
| 238.3 | (6.263 ± 0.510)e-03 | 0.88 ± 0.020 | 0.76 ± 0.024 | 1.03 ± 0.01 | 2.62 | 1.00 ± 0.003 | 5.919e-04 |
| 275.0 | (4.812 ± 0.410)e-03 | 0.96 ± 0.022 | 0.78 ± 0.022 | 1.01 ± 0.01 | 3.58 | 1.00 ± 0.004 | 4.810e-04 |
| 311.7 | (2.145 ± 0.163)e-03 | 0.96 ± 0.019 | 0.82 ± 0.018 | 1.01 ± 0.01 | 2.19 | 1.00 ± 0.004 | 1.823e-04 |
| 348.3 | (8.714 ± 0.848)e-04 | 0.95 ± 0.019 | 0.78 ± 0.022 | 1.01 ± 0.01 | 2.65 | 1.01 ± 0.006 | 9.344e-05 |
| 383.3 | (4.430 ± 0.616)e-04 | 0.92 ± 0.018. | 0.71 ± 0.029 | 1.02 ± 0.01 | 3.94 | 1.02 ± 0.009 | 6.733e-05 |
| 450.0 | (1.455 ± 0.221)e-04 | 1.03 ± 0.021 | 0.71 ± 0.029 | 1.01 ± 0.01 | 6.62 | 1.02 ± 0.010 | 2.504e-05 |

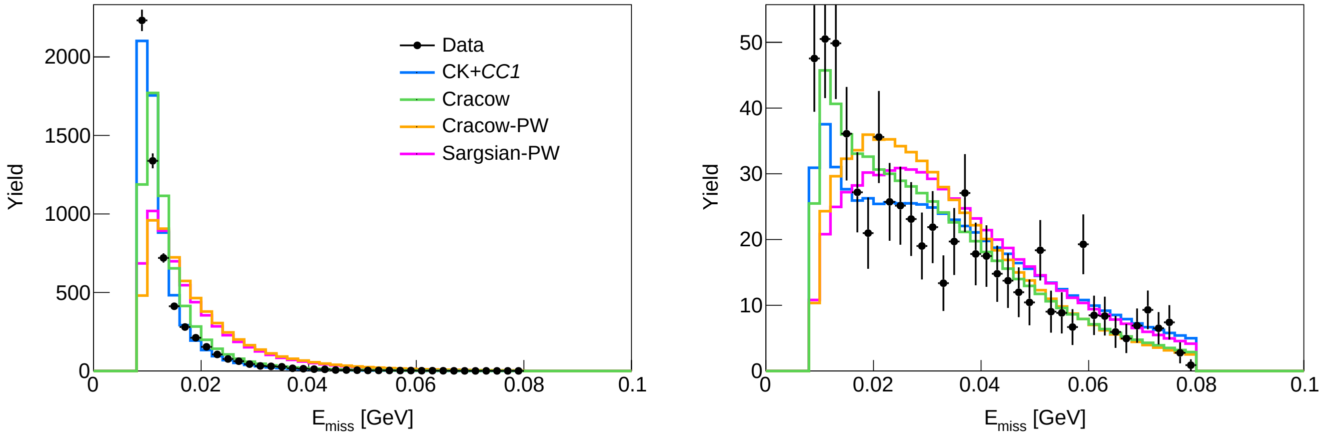


FIG. 10: $^{3}$He missing energy distribution for the low-$p_{miss}$ (left) and high-$p_{miss}$ (right) kinematical settings respectively. The corresponding $^{3}$H distributions are qualitatively very similar. The CK+$CC1$ (blue) and Cracow (green) curves include the continuum interaction between the two spectator nucleons (FSI$_{23}$) and the Cracow-PW (orange) and Sargsian-PW (magenta) curves do not. The FSI$_{23}$ effects are larger in the low-$p_{miss}$ kinematical setting.
